# Supplementary material for: A Formal Approach for Tuning Stochastic Oscillators
Source: arXiv:2405.09183 source file (2024-05-15)
Supplement: Supplementary file 1 [file appendix.tex]

\section{Further experiments}
\label{appendix:casestudies}
%\subsection{3-way sustained oscillator}
\begin{figure}[ht]

    \centering
    \begin{tabular}{cc}
    \includegraphics[width=0.5\textwidth]{ETFA21_paper/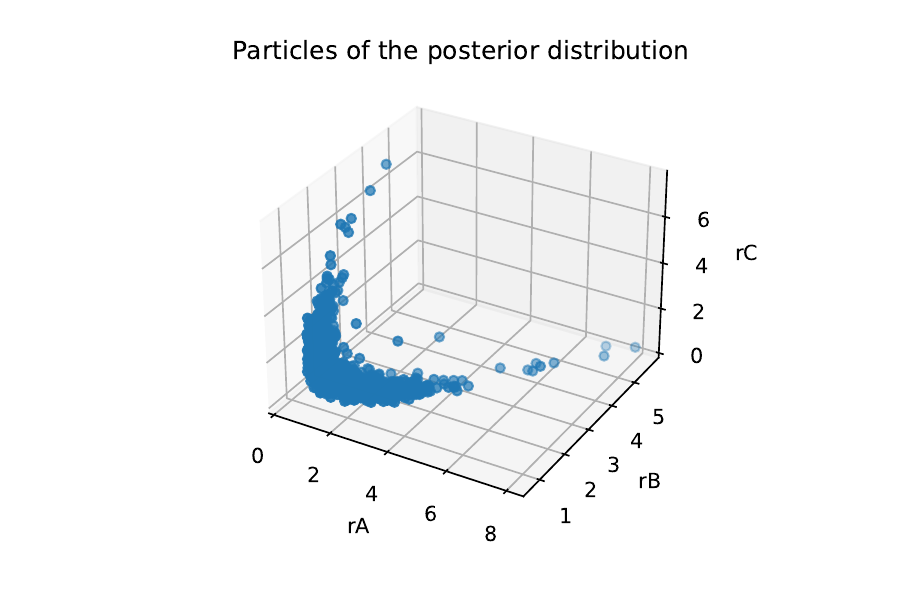}     & 
    \includegraphics[width=0.5\textwidth]{ETFA21_paper/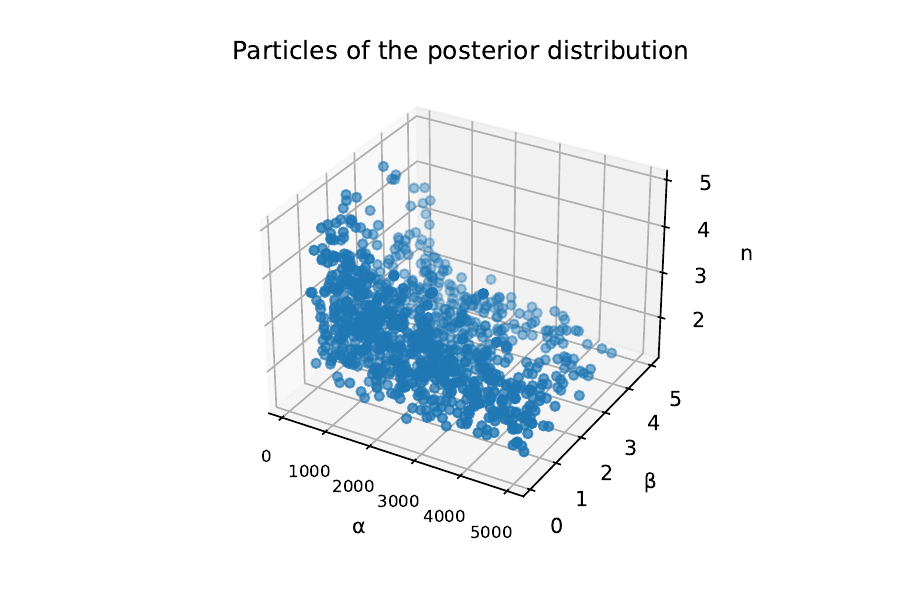}\\

    \end{tabular}
    
    \caption{Parapoloid-shaped support of the joint posterior distribution for the 3-dimensional parameter inference for the 3-way oscillator (left) and .}
    \label{fig:3way_3d_jointposterior}
\end{figure}

\subsection{Repressilator: a 4-dimensional experiment} 
\label{sec:repressilator}
{\bf Effect of parameters on the oscillation character}. Figure~\ref{fig:sim_repr_all} highlights the effect that each of the 4 parameters of the Repressilator model has on the resulting oscillatory character. Plots in the first row of of Figure~\ref{fig:sim_repr_all} refer to different values of $\alpha$ while $(\beta,n,\alpha_0)=(2,2,0)$, while in the second row $\beta$ is varied, in the third $\alpha_0$ is varied while in the bottom row $n$ is varied. 
Notice that amongst the chosen values,  $n$ has more influence on the stability of oscillations since simulations with $n = 0.5$ and $n = 1.0$ are very noisy.
Oscillations with $\alpha_0 = 0.0$ or $\alpha_0 = 0.01$ are quite stable. With $\alpha_0 = 0.1$, stability gets worst whereas simulations with $\alpha_0 = 1.0$ oscillations are much noisier. 
This remark is consistent with the stability diagram from \cite[Figure 1a.]{Elowitz2000}. Considering the continuous ODE model, they deduced the system is steady-state unstable if $\frac{\alpha}{\alpha_0} \geq 10^{-3}$, which is the case for $\alpha_0 = 1.0$ (as $\alpha = 200.0$).\\

\noindent
{\bf Approximated 3D support set for 3-way oscillator and the repressilator.}
Figure~\ref{fig:3way_3d_jointposterior} depicts the support set of the posterior-distribution for the 3-way oscillator (left) and for the Repressilator (right) corresponding to Experiment 2 (of the 3-way oscillator) and Experiment 1 (of the Repressilator). Notice the quire narrow paraboloid shaped form of the the support for the 3-way oscillator, denoting that the chosen target period $\obsmeantp = 0.01$ is ``matched'' only by relatively few combinations of parameters. \\% tthe 
\begin{figure}[ht]
    \centering
    \includegraphics[width=0.8\textwidth]{ETFA21_paper/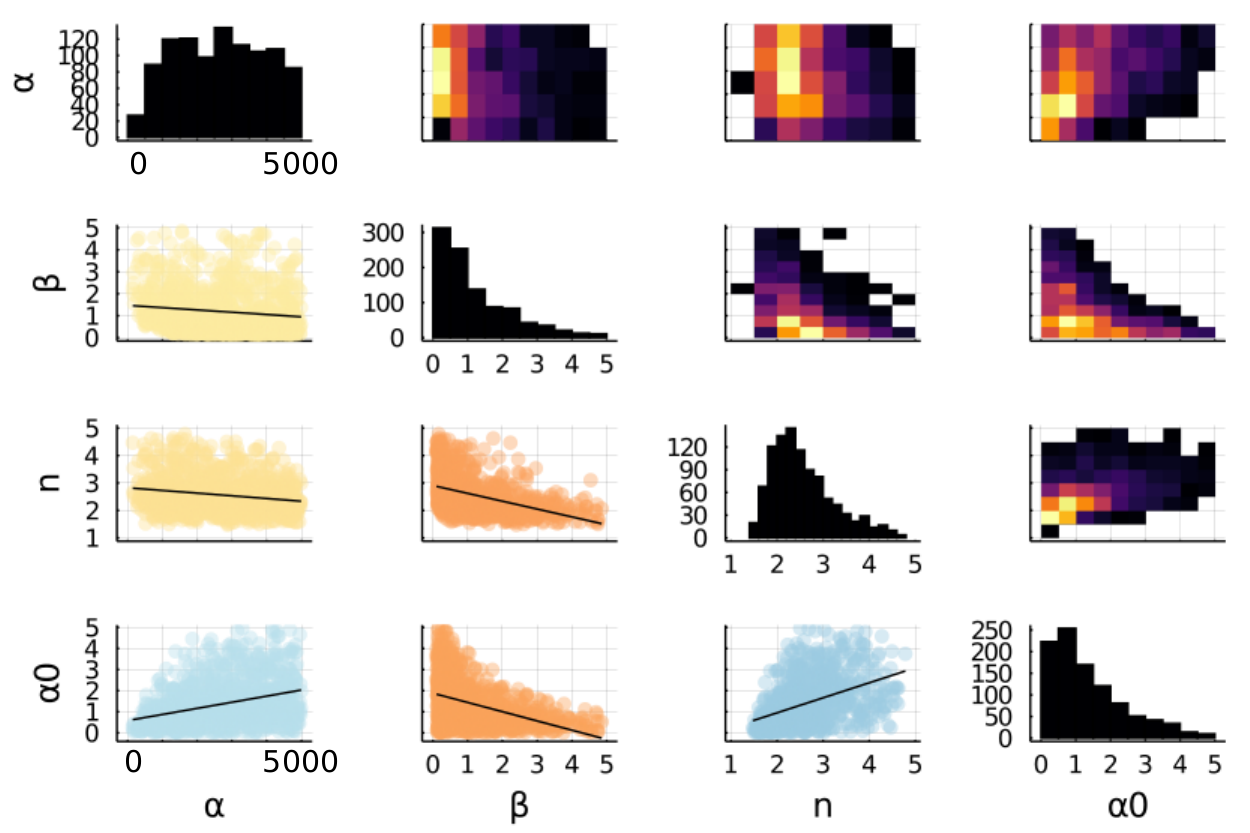}
    \caption{Correlation plot of automaton-ABC posterior with $\aut{per}$ posterior for the 4D experiment of repressilator model.}
    \label{fig:repressilator_4d_abc}
\end{figure}
%%%%%%%%%%%%%%%%%%%%%%%%%%%%%
\noindent{\bf Experiment 2}. 
This  is a 4-dimensional version of the previous  experiment in which we  considered also a uniform prior for $\beta \sim \Unif{0.1}{5.0}$. 
Figure~\ref{fig:repressilator_4d_abc} shows the correlation plot of the resulting automaton-ABC posterior. The parallel run (250 jobs) performed 22291 simulations and lasted 491 seconds. 
One can see adding a degree of freedom on $\alpha_0$ has changed the correlation between $\alpha$ and $\beta$ as well as $\alpha$ and $n$ whereas correlation between $\beta$ and $n$ seems to have the same shape.

%Figure~\ref{fig:sim_repr_alpha},  Figure~\ref{fig:sim_repr_beta}, Figure~\ref{fig:sim_repr_n} and Figure~\ref{fig:sim_repr_alpha0} depict paths corresponding to different configurations of  the Repressilator model. The default parameter values are $(\alpha, \beta, n, \alpha_0) = (200.0, 2.0, 2.0, 0.0)$, then each picture correspond to variations of one parameter only while the remaining three are kept as in the default setting. 

%Figure~\ref{fig:sim_repr_alpha} and Figure~\ref{fig:sim_repr_beta} show simulations with different parameter values of $\alpha$ and $\beta$. It illustrates trajectories with different amplitudes and period duration, but oscillations are pretty stable.

\begin{figure}[ht]
\begin{tabular}{cc}
\centering
  \includegraphics[width=0.5\textwidth]{ETFA21_paper/pic/sim_repressilator_alpha_1000_4000.png}   & \includegraphics[width=0.5\textwidth]{ETFA21_paper/pic/sim_repressilator_alpha_50_200.png}  \\
  \includegraphics[width=0.5\textwidth]{ETFA21_paper/pic/sim_repressilator_beta_0p5_1.png}   & \includegraphics[width=0.5\textwidth]{ETFA21_paper/pic/sim_repressilator_beta_2_4.png.png}  \\
\includegraphics[width=0.5\textwidth]{ETFA21_paper/pic/sim_repressilator_alpha0_0_001.png}   & \includegraphics[width=0.5\textwidth]{ETFA21_paper/pic/sim_repressilator_alpha0_01_1.png}  \\
\includegraphics[width=0.5\textwidth]{ETFA21_paper/pic/sim_repressilator_n_05_1.png}   & \includegraphics[width=0.5\textwidth]{ETFA21_paper/pic/sim_repressilator_n_2_5.png.png}  \\
\end{tabular}
\caption{Effect of the Repressilator's parameters on oscillations.}
    \label{fig:sim_repr_all}
\end{figure}

\section{HASL model checking}
\label{appendix:hasl}

\subsection{Hybrid automaton as property specification}
%{\bf Hybrid automaton as property specification}. 
With HASL model checking   a LHA ${\cal A}$ is employed as a \emph{path selector} through synchronisation with the considered model ${\cal M}$. An automaton ${\cal A}$  has access to certain elements of model ${\cal M}$, namely the events (i.e. the reactions of the CRN) and the state-variables of ${\cal M}$. Formally a LHA  for HASL is  defined as an $n$-tuple: 
$$
 \mathcal A=\langle E, L, V, \Lambda, \init, \final, \flow, \rightarrow \rangle
$$
\noindent
where:
$E$ is a finite alphabet of events (the reactions of the CRN model);  $L$ is a finite set of locations; $V=(v_1,...v_n)$ a $n$-tuple of data variables; $\Lambda: L \rightarrow Prop$, a location labelling function ($\mathit{Prop}$ being the set of atomic proposition built on top of variables $V$); $\init\subset L$ ($\final\subset L$) is the set of  initial (final) locations;   $\flow : L \mapsto Ind^n$ characterises  the rate at which each variable $v_i$ evolves in each location (where the rate for variable $v_i$ is given by an \emph{indicator function} that depends on the state of the model ${\cal M}_\theta$); $\rightarrow \subseteq L \times   \left( (\const \times 2^E) \uplus (\lconst \times \{\sharp\}) \right) \times \updates \times L$, a set of edges, where the notation $l\xrightarrow{\gamma,E',U}l'$ means that $(l,\gamma,E',U,l') \in \rightarrow$, with \
 $\const$ the set of constraints, whose elements are  Boolean combinations of inequalities 
of the form $\sum_{1 \leq i \leq n}\aconst_i v_i +c \prec 0$ where $\aconst_i$ and $c$ are constants,
$\prec\in\!\{=, <, >, \leq, \geq\}$, whereas $\lconst$ is the set of left-closed constraints. 
Selection of a model's trajectories with an automaton ${\cal A}$ is achieved through \emph{synchronization} of ${\cal M}$ with ${\cal A}$, i.e. by letting ${\cal A}$ synchronises its transitions with the transitions of the trajectory $\sigma$ being sampled. To this aim, an LHA for HASL admits two kinds of transitions: \emph{synchronizing} transitions (associated with a subset $E\subseteq \Sigma$ of event names, with $\mathit{ALL}$ denoting $\Sigma$), which may be traversed when an event (in $E$) is observed on $\sigma$ (for example a reaction occurs), and \emph{autonomous} transitions (denoted by $\sharp$) which are traversed autonomously (and have priority over synchronised transitions), on given conditions, typically to update relevant statistics or to terminate (accept) the analysis of $\sigma$. 

\subsection{Synchronisation of a DESP model with a LHA}. 

\medskip
The synchronisation of  ${\cal M}$ with  ${\cal A}$  boils down to the characterisation of the  product process ${\cal M}\times{\cal A}$ whose semantics we describe intuitively here (referring the reader to  ~\cite{BALLARINI201553} for its formal characterisation).
For  ${\cal M}$ a DESP with state space $S$ and  ${\cal A}$ a LHA with  locations $L$ and  variables $V$ the states of ${\cal M}\times{\cal A}$ are triples 
$(s,l,\nu)$
where $s\in S$ is the current state of ${\cal M}$, $l\in L$ is the current location of ${\cal A}$ and $\nu:V\to\mathbb{R}^{|V|}$ is the current value of of the variables of ${\cal A}$. 
The semantics of ${\cal M}\times{\cal A}$ naturally yields a stochastic simulation procedure which is implemented by the HASL model checker. The paths of ${\cal M}\times{\cal A}$ sampled by the HASL simulator are composed of two kinds of transitions: \emph{synchronising transitions}, that correspond to a simultaneous  occurrence of a transition in ${\cal M}$ and one in ${\cal A}$, as opposed to, \emph{autonomous transitions},   that correspond to the occurrence  of a transition in ${\cal A}$ without any correspondence in ${\cal M}$. 
Therefore a path of ${\cal M}\times{\cal A}$ can be seen as the result of the synchronisation of a path $\sigma$ of ${\cal M}$ with ${\cal A}$ (or conversely we may say that a path of ${\cal M}\times{\cal A}$ always admits a projection over ${\cal M}$). Given $\sigma$ a path of ${\cal M}$ we denote  $\sigma\times{\cal A}$ the corresponding path of  ${\cal M}\times{\cal A}$. For example if 
$
\sigma: s\xrightarrow[e_1]{t_1}s_1\xrightarrow[e_2]{t_2}s_2\ldots 
$
is a path of ${\cal M}$ such that after sojourning for $t_1$ in its origin  state $s$, switches to $s_1$ through occurrence of event $e_1$, and then, at $t_2$, switches to $s_2$, through event $e_2$ (and so on), then the corresponding path  $\sigma\times{\cal A}$ in the product process may be
$
\sigma\times{\cal A}: (s,l,\nu)\xrightarrow[e_1]{t_1}(s_1,l_1,\nu_1)\xrightarrow[\sharp]{t^*_1}(s_1,l_2,\nu_2)\xrightarrow[e_2]{t_2}(s_2,l_3,\nu_3)\ldots 
$
where, the sequence of transitions $e_1$ and $e_2$ observed on $\sigma$ is interleaved with an autonomous transition (denoted $\sharp$) in the product process: i.e. from state $(s_1,l_1,\nu_1)$ the product process jumps to state $(s_1,l_2,\nu_2)$ (notice that state of ${\cal M}$ does not change) before continuing mimicking $\sigma$. The semantics of the product process is detailed in Example~\ref{ex1}. 

\subsection{HASL target expression $Z$}
\noindent
{\bf HASL target expression.} The second component of an HASL specification is an expression $Z$ given by grammar~(\ref{haslexp}). $Z$ is associated to   a LHA ${\cal A}$ and  expresses the target measure whose confidence interval should be estimated based on the paths accepted by ${\cal A}$. \\
\begin{footnotesize}
  \begin{equation}
  \label{haslexp}
  \begin{split}
 Z  & ::=  \ AVG(Y)\ |\ Z+Z\ |\ Z \times Z \ |\ Pdist\\
 Pdist  & ::=  \ PDF(Y,step,start,stop))\ |\  {CDF(Y,step,start,stop)}\ |\  {PROB()}\\
 Y  & ::= \ c\ |\ Y+Y\ |\ Y \times Y\ |\ Y/Y\ |\ {last(y)}\ |\ min(y)\  \  |\ {max(y)}\\% |\ {int(y)}\ |\ {avg(y)}\\
% \label{truc}
 y  & ::= \ c\ |\ x\ |\ y+y\ |\ y \times y\ |\ y/y    
  \end{split}
  \end{equation}
\end{footnotesize}  
There are two main types of expressions $Z$:  $AVG(Y)$ (where $AVG$ indicates \emph{mean value of}) and $Pdist$  (indicating a probability distribution or probability value expression). $Y$ represent a random variable built on top of algebraic combination of some \emph{path} operators applied to an LHA variable $y$, i.e. $last(y)$ (i.e. the last value that   $y$ has at the end of an accepted path, $min(y) (resp. $max(y)$)$, the min (resp. max) value of $y$ along an accepted path. Conversely $Z$ expressions of $Pdist$ type include $PDF(Y,step,start,stop)$, which allows for estimating the PDF of random variable $Y$ computed by discretisation of the support set $[start,stop]$ in $(stop-start)/step$   sub-intervals of size $step$ and similarly  $CDF(Y,step,start,stop)$, Finally expression $PROB()$ allows for estimating the probability that a path is accepted, otherwise said $PROB()$ is used to estimating the probability of the paths event set represented by the considered automaton ${\cal A}$. 
\subsection{Variables of the  $\autpertpobs$ automaton}
The complete list of data variables of the $\autpertpobs$ automaton is given in Table~\ref{tab:lhavars2_complete}. 
\begin{table}[ht]
    \centering\footnotesize
    \begin{tabular}{|c|c|c|p{4.5cm}|}
           \hline
    {\bf name} & {\bf domain}  & {\bf update definition} & {\bf description}  \\ \hline
     
        $t$ & $\mathbb{R}_{\geq 0}$ & \emph{reset} & time elapsed since beginning measure (first non-spurious period) \\ \hline
      $n$ & $\mathbb{N}$ & \emph{increment} & counter of  detected periods \\ \hline
      $n_A$ & $\mathbb{N}$ & $n_A=A$ & current population of the periodic species \\ \hline
      $top$ & bool & \emph{complement} & boolean flag indicating whether the high part of the partition has been entered \\ \hline
   
    $n$ & $\mathbb{N}$ & \emph{increment} & counter of  detected periods \\ \hline
    ${t}_p$ & $\mathbb{R}_{\geq 0}$ &  \emph{reset}  & duration  last  period  \\ \hline    
        $\bar{t}_p$ & $\mathbb{R}_{\geq 0}$ & $  f(\bar{t}_p,t_p,n)=\frac{\bar{t}_{p_n}\cdot n+t_p}{n+1}$ & period mean \\ \hline
   $s^2_{t_p}$ & $\mathbb{R}_{\geq 0}$ & $g(s^2_{t_{p}},\bar{t}_p,t_p,n)  =
    \frac{n-1}{n-2}\cdot s^2_{t_{p}}+\frac{(\bar{t}_p-t_p)^2}{n-1}$    & period variance      \\          \hline         
    $d_p$ & $\mathbb{R}_{\geq 0}$ & 
    $\min(\frac{\meantp-\obsmeantp}{\obsmeantp},\frac{\sqrt{\vartp}}{\obsmeantp})$ & distance from target period      \\         
    \hline 
    \end{tabular}
    \caption{ Variables  of the  $\autpertpobs$ automaton. }
    \label{tab:lhavars2_complete}
    \end{table}

\begin{algorithm}
    \begin{algorithmic}
        \REQUIRE $\mcpCTMC$ parametric CTMC, $\pi$ prior,
        \\$N$: number of particles, $\eps$: tolerance level, $\alpha$: quantile level,
        \\$Y$ HASL trajectory expression, ${\cal A}$ LHA, $K$: kernel proposal density
        \ENSURE $(\omega^{(i)}, \theta^{(i)})_{1 \leq i \leq N}$ weighted samples drawn from $\pi^\epsilon_{ABC}$ %$\piabceps$
        \STATE $\theta_0^{(i)} \sim \pi, i \in {1,\ldots, N}$
        \STATE $d_i \sim (Y,\aut ) \times \mcCTMC[\theta^{(i)}_0], 0 \in {1,\ldots, N}$
        \STATE $\epsilon \gets quantile(\alpha, (d_i)_{1 \leq i \leq N})$
        \STATE $(\omega_0^{(i)})_{1 \leq i \leq N} \gets \frac{1}{N}$
        \STATE $m \gets 1$
        \WHILE{$\epsilon > 0$}
        \FOR{$i = 1:N$}
        \REPEAT
        \STATE Take $\theta'$ from $(\theta_{m-1}^{(j)})_{1 \leq j \leq N}$ with probabilities $(\omega_{m-1}^{(j)})_{1\leq j\leq N}$
        \STATE $\theta_m^{(i)} \sim K(.|\theta')$
        \STATE $d_i \sim (Y,\aut) \times \mcCTMC[\theta_m^{(i)}]$
        \UNTIL{$d_i \leq \epsilon$}
        \STATE $\omega^{(i)}_m \gets \frac{\pi\left(\theta_m^{(i)} \right)}{
        \overset{N}{\underset{i'=1}{\Sigma}}  \omega_{m-1}^{(i')} K(\theta_m^{(i)} | \theta_{m-1}^{(i')})}$
        \ENDFOR
        \STATE Normalise $(\omega_m^{(i)})_{1\leq i\leq N}$
        \STATE $\epsilon \gets quantile(\alpha, (d_i)_{1 \leq i \leq N})$
        \STATE $m \gets m+1$
        \ENDWHILE
         \RETURN $(\omega^{(i)}_m, \theta^{(i)}_m)_{1 \leq i \leq N}$
    \end{algorithmic}
    \caption{General automaton-ABC Sequential Monte Carlo Algorithm}
    \label{alg:general_automaton_abc_smc}
\end{algorithm}

\section{HASL-based Sequential Monte Carlo ABC method}
\label{appendix:abcsmchasl}
%\label{sec:appendix}
Algorithm~\ref{alg:general_automaton_abc_smc} is the Sequential Monte Carlo version of Algorithm~\ref{alg:general_automaton_abc}.
